# Supplementary material for: Carrier diffusion in semiconductor nanoscale resonators
Source: arXiv:2308.16715 ancillary file (2023-08-31)
Supplement: Supplementary file 1 [file Carrier_diffusion_ArXiV_2028-08-31_SUPPLEMENTARY_submitted.pdf]

# Supplementary material for "Carrier diffusion in semiconductor nanoscale resonators"

Marco Saldutti, Yi Yu, George Kountouris, Philip Trøst Kristensen and Jesper Mørk  
*DTU Electro, Technical University of Denmark, DK-2800 Kgs. Lyngby, Denmark and*  
*NanoPhoton - Center for Nanophotonics, Technical University of Denmark, DK-2800 Kgs. Lyngby, Denmark*  
 (Dated: August 31, 2023)

## I. DETAILS ON THE EIGENMODE EXPANSION AND RESPONSE FUNCTION FORMALISM

The starting point is the ambipolar diffusion equation [1]:

$$\frac{\partial N(\mathbf{r}, t)}{\partial t} = D_{\text{eff}} \nabla^2 N(\mathbf{r}, t) - \frac{N(\mathbf{r}, t)}{\tau_{\text{bulk}}} + G(\mathbf{r}, t) \quad (1)$$

Here,  $N(\mathbf{r}, t)$  is the excess carrier density with respect to thermal equilibrium, hereafter simply denoted by carrier density. The nonradiative recombination lifetime,  $\tau_{\text{bulk}}$ , reflects Shockley-Read-Hall (SRH) recombination in the bulk semiconductor material. At typical carrier densities around  $10^{15} \sim 10^{18} \text{ cm}^{-3}$ , radiative and Auger recombination in III-V semiconductors are usually characterized by longer lifetimes [2, 3].  $G(\mathbf{r}, t)$  is the carrier generation rate per unit time and unit volume, and  $D_{\text{eff}}$  is the ambipolar diffusion coefficient.

Eq. 1 is complemented by Neumann boundary conditions

$$D_{\text{eff}} \hat{\mathbf{n}} \cdot \nabla N(\mathbf{r}, t) = -v_s N(\mathbf{r}, t) \quad (2)$$

modeling SRH recombination at the interface between the semiconductor and the surrounding dielectric material. Here,  $v_s$  is the surface recombination velocity, scaling with the density of surface states, and  $\hat{\mathbf{n}}$  is the unit vector normal to the surface and pointing outwards.

We expand the carrier density as

$$N(\mathbf{r}, t) = \sum_i c_i(t) R_i(\mathbf{r}) \quad (3)$$

Here,  $R_i(\mathbf{r})$  are the eigenmodes of the eigenvalue equation

$$D_{\text{eff}} \nabla^2 R_i(\mathbf{r}) = -\gamma_i R_i(\mathbf{r}) \quad (4)$$

with boundary conditions

$$D_{\text{eff}} \hat{\mathbf{n}} \cdot \nabla R_i(\mathbf{r}) = -v_s R_i(\mathbf{r}) \quad (5)$$

and  $\gamma_i$  are the eigenvalues. Importantly, since the Laplacian operator in Eq. 4 is Hermitian, the eigenvalues are real, while the eigenmodes are orthogonal and form a complete basis set [4]. The Hermitian nature

of the Laplacian operator readily follows from Green's second identity

$$\int_{V_m} [R_i(\mathbf{r}) \nabla^2 R_j(\mathbf{r}) - R_j(\mathbf{r}) \nabla^2 R_i(\mathbf{r})] d^3 \mathbf{r} = \int_{\Phi} [R_i(\mathbf{r}) \hat{\mathbf{n}} \cdot \nabla R_j(\mathbf{r}) - R_j(\mathbf{r}) \hat{\mathbf{n}} \cdot \nabla R_i(\mathbf{r})] d\Phi \quad (6)$$

where  $V_m$  is the semiconductor volume and  $\Phi$  is the surface enclosing it. The right-hand side of Eq. 6 vanishes as a result of Eq. 5, implying that the Laplacian operator is Hermitian.

We assume the carrier generation rate to be a separable function in the form

$$G(\mathbf{r}, t) = F(\mathbf{r}) f(t) \quad (7)$$

In particular, for carriers generated via **two-photon absorption** [5–7], one finds

$$F(\mathbf{r}) = |\mathbf{E}(\mathbf{r})|^4 \quad (8)$$

where  $\mathbf{E}(\mathbf{r})$  is the electric field of the cavity mode.

By inserting Eq. 3 into Eq. 1 and utilizing Eq. 4, we obtain

$$\sum_i \left[ R_i(\mathbf{r}) \frac{dc_i(t)}{dt} + \left( \gamma_i + \frac{1}{\tau_{\text{bulk}}} \right) R_i(\mathbf{r}) c_i(t) \right] = F(\mathbf{r}) f(t) \quad (9)$$

Then, we multiply both sides by  $R_j(\mathbf{r})$  and integrate over the semiconductor volume. The orthogonality of the eigenmodes, namely

$$\int_{V_m} R_i(\mathbf{r}) R_j(\mathbf{r}) d^3 \mathbf{r} = \delta_{ij} \int_{V_m} R_i^2(\mathbf{r}) d^3 \mathbf{r} \quad (10)$$

with  $\delta_{ij}$  being the Kronecker delta, leads to

$$\frac{dc_i(t)}{dt} + \frac{c_i(t)}{\tau_i} = A_i f(t) \quad (11)$$

where the lifetime  $\tau_i$  is given by

$$\frac{1}{\tau_i} = \gamma_i + \frac{1}{\tau_{\text{bulk}}} \quad (12)$$

and the coefficient  $A_i$  reads

$$A_i = \frac{\int_{V_m} R_i(\mathbf{r}) F(\mathbf{r}) d^3 \mathbf{r}}{\int_{V_m} R_i^2(\mathbf{r}) d^3 \mathbf{r}} \quad (13)$$

The eigenmode expansion has conveniently reduced the ambipolar diffusion equation (a partial differential equation in space and time) to a set of ordinary differential equations in time only. Eq. 11 is readily solvable if the eigenmodes,  $R_i(\mathbf{r})$ , and the eigenvalues,  $\gamma_i$ , are known.

### A. Free evolution

We start considering the **free evolution**. In this case, one finds  $f(t) = 0$ , and  $N(\mathbf{r}, t)$  evolves in time from the initial condition,  $N(\mathbf{r}, t=0) = F(\mathbf{r})$ .

From Eq. 11 and Eq. 3, one readily finds

$$N(\mathbf{r}, t) = \sum_i c_i(t=0) R_i(\mathbf{r}) e^{-\frac{t}{\tau_i}} \quad (14)$$

Imposing the initial condition on  $N(\mathbf{r}, t)$  leads to  $N(\mathbf{r}, t=0) = \sum_i c_i(t=0) R_i(\mathbf{r}) = F(\mathbf{r})$ . Then, multiplying both sides by  $R_j(\mathbf{r})$ , integrating over the semiconductor volume and exploiting Eq. 10, one readily finds

$$c_i(t=0) = A_i \quad (15)$$

### B. Forced evolution

We now consider the **forced evolution**, whereby the initial condition is null, and it is  $f(t)$  which drives the time evolution of the carrier density.

Eq. 11 can be readily solved by using the Laplace transform technique. Transforming the left- and right-hand side gives  $c_i(s) = A_i \frac{f(s)}{s+1/\tau_i}$ , with  $c_i(s)$  and  $f(s)$  being the Laplace transform of  $c_i(t)$  and  $f(t)$ , respectively. Subsequent application of the inverse Laplace transform leads to

$$c_i(t) = A_i \int_0^t f(\tau) e^{-\frac{t-\tau}{\tau_i}} d\tau \quad (16)$$

Hence, the carrier density from Eq. 3 can be expressed as

$$N(\mathbf{r}, t) = \int_0^t f(\tau) h(\mathbf{r}, t-\tau) d\tau \quad (17)$$

Here,  $h(\mathbf{r}, t)$  reads

$$h(\mathbf{r}, t) = \sum_i A_i R_i(\mathbf{r}) e^{-\frac{t}{\tau_i}} \quad (18)$$

and is the response function of the carrier density. Indeed, for  $f(t) = \delta(t)$ , with  $\delta(t)$  being the Dirac delta, the convolution integral in Eq. 17 readily gives  $N(\mathbf{r}, t) = h(\mathbf{r}, t)$ .

Importantly, we note that the response function coincides with the free evolution (cf. Eq. 14). Therefore, solving the ambipolar diffusion equation with  $G(\mathbf{r}, t) = 0$  and initial condition  $N(\mathbf{r}, t=0) = F(\mathbf{r})$  provides the response function, independently of the solution technique.

### C. Effective carrier density

Within the framework of coupled-mode theory, the shift in the cavity resonance induced by the generated carriers scales to first order with a mode-averaged or **effective carrier density** [6–8]

$$N_{\text{eff}}(t) = \frac{\int_{V_m} N(\mathbf{r}, t) \epsilon(\mathbf{r}) |\mathbf{E}(\mathbf{r})|^2 d^3\mathbf{r}}{\int_V \epsilon(\mathbf{r}) |\mathbf{E}(\mathbf{r})|^2 d^3\mathbf{r}} \quad (19)$$

Here,  $\epsilon(\mathbf{r})$  is the permittivity and  $V$  is an integration volume enclosing the optical cavity with a margin of a few wavelengths.

We first consider the **free evolution**, and insert Eq. 14 into Eq. 19. This provides

$$N_{\text{eff}}(t) = \sum_i \kappa_i e^{-\frac{t}{\tau_i}} \quad (20)$$

where the excitation coefficient,  $\kappa_i$ , reads

$$\kappa_i = A_i \frac{\int_{V_m} R_i(\mathbf{r}) \epsilon(\mathbf{r}) |\mathbf{E}(\mathbf{r})|^2 d^3\mathbf{r}}{\int_V \epsilon(\mathbf{r}) |\mathbf{E}(\mathbf{r})|^2 d^3\mathbf{r}} \quad (21)$$

As for the **forced evolution**, by combining Eq. 17 with Eq. 19, we obtain

$$N_{\text{eff}}(t) = \int_0^t f(\tau) h_{\text{eff}}(t-\tau) d\tau \quad (22)$$

where the response function of the effective carrier density,  $h_{\text{eff}}(t)$ , reads

$$h_{\text{eff}}(t) = \sum_i \kappa_i e^{-\frac{t}{\tau_i}} \quad (23)$$

Again, we note that the response function coincides with the free evolution, Eq. 20.

## II. IN-PLANE AND OUT-OF-PLANE EIGENVALUE PROBLEMS

As illustrated in Sec. I, the free evolution of the ambipolar diffusion equation determines the response function. In the following, we show that the carrier diffusion dynamics, and hence the response function, can be effectively separated into a contribution due to two-dimensional, **in-plane diffusion**, and another driven

by one-dimensional, **out-of-plane diffusion** along the cavity growth direction.

We consider the homogeneous (source-free) ambipolar diffusion equation

$$\frac{\partial N(\mathbf{r}, t)}{\partial t} = D_{\text{eff}} \nabla^2 N(\mathbf{r}, t) - \frac{N(\mathbf{r}, t)}{\tau_{\text{bulk}}} \quad (24)$$

with parameters defined as in Sec. I, with initial condition given by  $N(\mathbf{r}, t = 0) = F(\mathbf{r})$ , and subject to surface recombination boundary conditions as described by Eq. 2. We postulate a solution in the form

$$N(\mathbf{r}, t) = R(\mathbf{r})T(t)e^{-\frac{t}{\tau_{\text{bulk}}}} \quad (25)$$

and plug it into Eq. 24, which leads to

$$\frac{1}{T(t)} \frac{dT(t)}{dt} = D_{\text{eff}} \frac{\nabla^2 R(\mathbf{r})}{R(\mathbf{r})} \quad (26)$$

Since the left- and right-hand sides only depend on time and position, respectively, they must be equal to the same constant for the equation to be fulfilled.

Denoting this constant by  $-\gamma$ , we find

$$T(t) = t_0 e^{-\gamma t} \quad (27)$$

with the coefficient  $t_0$  to be determined from the initial condition. As for the spatial dependence, we obtain the eigenvalue equation

$$D_{\text{eff}} \nabla^2 R(\mathbf{r}) = -\gamma R(\mathbf{r}) \quad (28)$$

that is identical to Eq. 4. Furthermore, upon insertion of Eq. 25, the boundary conditions in Eq. 2 provide

$$D_{\text{eff}} \hat{\mathbf{n}} \cdot \nabla R(\mathbf{r}) = -v_s R(\mathbf{r}) \quad (29)$$

which coincides with Eq. 5. With considerations analogous to Sec. I (the Laplacian operator of the eigenvalue problem is Hermitian), one could expand  $R(\mathbf{r})$  on the eigenmodes and obtain the solution, Eq. 14.

Here, instead, we further postulate a solution in the form

$$R(\mathbf{r}) = u(\mathbf{r}_{\parallel})v(z) \quad (30)$$

with  $\mathbf{r}_{\parallel}$  being the in-plane position vector and  $z$  the out-of-plane position coordinate. We emphasize that for the solution to be exact, the initial condition must also be separable, namely

$$F(\mathbf{r}) = F_{\text{xy}}(\mathbf{r}_{\parallel})F_z(z) \quad (31)$$

which is **not** necessarily the case. However, as illustrated in the main text, we have found Eq. 31 and, therefore, Eq. 30, to be effective approximations.

Upon insertion of Eq. 30 into Eq. 28, we find

$$D_{\text{eff}} \frac{\nabla_{\parallel}^2 u(\mathbf{r}_{\parallel})}{u(\mathbf{r}_{\parallel})} + \frac{D_{\text{eff}}}{v(z)} \frac{d^2 v(z)}{dz^2} = -\gamma \quad (32)$$

For the equation to be fulfilled, the two addends on the left-hand side must be separately equal to constants, with the two constants being generally different. Hence, we find an eigenvalue equation for the in-plane diffusion

$$D_{\text{eff}} \nabla_{\parallel}^2 u(\mathbf{r}_{\parallel}) = -\gamma_{\text{xy}} u(\mathbf{r}_{\parallel}) \quad (33)$$

and another for the out-of-plane diffusion

$$\frac{d^2 v(z)}{dz^2} = -\alpha_z^2 v(z) \quad (34)$$

with the eigenvalues fulfilling

$$\gamma = \gamma_{\text{xy}} + D_{\text{eff}} \alpha_z^2 \quad (35)$$

The boundary conditions are readily found upon insertion of Eq. 30 into Eq. 29, which provides

$$D_{\text{eff}} \hat{\mathbf{n}}_{\parallel} \cdot \nabla_{\parallel} u(\mathbf{r}_{\parallel}) = -v_s u(\mathbf{r}_{\parallel}) \quad (36)$$

for the in-plane diffusion and

$$\pm D_{\text{eff}} \frac{dv(z)}{dz} \Big|_{z=\pm \frac{L_z}{2}} = -v_s v(z) \Big|_{z=\pm \frac{L_z}{2}} \quad (37)$$

for the out-of-plane diffusion, with  $L_z$  being the cavity thickness along the growth direction. Here, we have assumed **symmetric** boundary conditions, i.e. the same surface recombination velocity at the top and bottom surface of the cavity. The more general case of **asymmetric** boundary conditions is addressed in Sec. III.

The Laplacian operator and the second-order derivative of the in-plane and out-of-plane eigenvalue problem, respectively, are both Hermitian. Therefore, we may express the total solution as

$$N(\mathbf{r}, t) = N_{\text{xy}}(\mathbf{r}_{\parallel}, t) N_z(z, t) e^{-\frac{t}{\tau_{\text{bulk}}}} \quad (38)$$

where the in-plane contribution,  $N_{\text{xy}}(\mathbf{r}_{\parallel}, t)$ , and the out-of-plane contribution,  $N_z(z, t)$ , read

$$N_{\text{xy}}(\mathbf{r}_{\parallel}, t) = \sum_i A_{\text{xy}_i} u_i(\mathbf{r}_{\parallel}) e^{-\gamma_{\text{xy}_i} t} \quad (39)$$

$$N_z(z, t) = \sum_j A_{z_j} v_j(z) e^{-D_{\text{eff}} \alpha_{z_j}^2 t} \quad (40)$$

Here,  $u_i(\mathbf{r}_{\parallel})$  and  $v_j(z)$  are the eigenmodes of the in-plane and out-of-plane eigenvalue problem, respectively, with  $\gamma_{\text{xy}_i}$  and  $\alpha_{z_j}^2$  being the corresponding eigenvalues. In the following, we fully derive the out-of-plane contribution.

The expansion coefficients,  $A_{z_j}$ , are found by enforcing the initial condition,  $N(\mathbf{r}, t = 0) = F_{xy}(\mathbf{r}_{\parallel})F_z(z)$ , and noting that  $N_{xy}(\mathbf{r}_{\parallel}, t = 0) = F_{xy}(\mathbf{r}_{\parallel})$  and  $N_z(z, t = 0) = F_z(z)$  must hold separately. Multiplying both sides of the latter equality by  $A_{z_l}$ , integrating over  $L_z$  and leveraging the orthogonality of the out-of-plane eigenmodes, we find

$$A_{z_j} = \frac{\int_{L_z} v_j(z) F_z(z) dz}{\int_{L_z} v_j^2(z) dz} \quad (41)$$

If both the boundary conditions (cf. Eq. 37) and the initial condition,  $F_z(z)$ , are **symmetric** with respect to  $z$ , then  $v_j(z)$  must be an even function of  $z$  and we may postulate

$$v_j(z) = \cos(\alpha_{z_j} z) \quad (42)$$

Hence, we may further develop  $A_{z_j}$  into

$$A_{z_j} = \frac{2\alpha_{z_j}}{\alpha_{z_j} L_z + \sin(\alpha_{z_j} L_z)} \int_{L_z} \cos(\alpha_{z_j} z) F_z(z) dz \quad (43)$$

The eigenvalues are found by inserting Eq. 42 into Eq. 37, which provides

$$\cot\left(\frac{\alpha_{z_j} L_z}{2}\right) = \left(\frac{2D_{\text{eff}}}{L_z v_s}\right) \left(\frac{\alpha_{z_j} L_z}{2}\right) \quad (44)$$

The equation is readily solvable, graphically or numerically.

By inserting Eq. 38 into Eq. 19, we finally arrive at the response function of the effective carrier density:

$$h_{\text{eff}}(t) = h_{\text{eff},xy}(t) h_{\text{eff},z}(t) e^{-\frac{t}{\tau_{\text{bulk}}}} \quad (45)$$

Here, the in-plane contribution,  $h_{\text{eff},xy}(t)$ , and the out-of-plane contribution,  $h_{\text{eff},z}(t)$ , have expressions analogous to Eq. 20, with obvious changes of volume integrals into surface and one-dimensional integrals, respectively, when computing the excitation coefficients. Furthermore, we have assumed the electric energy density,  $\epsilon(\mathbf{r})|\mathbf{E}(\mathbf{r})|^2$ , to be a separable function of  $\mathbf{r}_{\parallel}$  and  $z$ , similarly to the initial condition (cf. Eq. 31).

### III. ASYMMETRIC OUT-OF-PLANE DIFFUSION

As illustrated in Sec. II, the free evolution of the ambipolar diffusion equation, and hence the response function, can be expressed as the product of two contributions, reflecting, respectively, in-plane diffusion and out-of-plane diffusion along the cavity growth direction,  $z$  (cf. Eq. 38 and Eq. 45). Furthermore, the case of symmetric out-of-plane diffusion has been treated explicitly.

In the following, we extend the treatment to the more general situation of **asymmetric** out-of-plane diffusion, whereby the boundary conditions or the initial condition,  $F_z(z)$  (cf. Eq. 31), are not symmetric with respect to  $z$ . The results herein derived are consistent with previous works [9, 10].

The boundary conditions read

$$D_{\text{eff}} \frac{dv(z)}{dz} \Big|_{z=+\frac{L_z}{2}} = -v_{s_t} v(z) \Big|_{z=+\frac{L_z}{2}} \quad (46)$$

$$-D_{\text{eff}} \frac{dv(z)}{dz} \Big|_{z=-\frac{L_z}{2}} = -v_{s_b} v(z) \Big|_{z=-\frac{L_z}{2}} \quad (47)$$

with  $v_{s_t}$  and  $v_{s_b}$  being the surface recombination velocity at the top and bottom surface, respectively. As already seen in Sec. II, the out-of-plane contribution to the carrier density,  $N_z(z, t)$ , is given by Eq. 40

$$N_z(z, t) = \sum_j A_{z_j} v_j(z) e^{-D_{\text{eff}} \alpha_{z_j}^2 t} \quad (48)$$

However, owing to the asymmetry, the eigenmodes,  $v_j(z)$ , are **not** even functions of  $z$ . In general, we may postulate

$$A_{z_j} v_j(z) = \alpha_{z_j} \cos(\alpha_{z_j} z) + \beta_{z_j} \sin(\alpha_{z_j} z) \quad (49)$$

Enforcing the boundary condition at the bottom surface leads to

$$D_{\text{eff}} \left[ \alpha_{z_j} \alpha_{z_j} \sin\left(\alpha_{z_j} \frac{L_z}{2}\right) + \beta_{z_j} \alpha_{z_j} \cos\left(\alpha_{z_j} \frac{L_z}{2}\right) \right] = v_{s_b} \left[ \alpha_{z_j} \cos\left(\alpha_{z_j} \frac{L_z}{2}\right) - \beta_{z_j} \sin\left(\alpha_{z_j} \frac{L_z}{2}\right) \right] \quad (50)$$

from which we find the ratio

$$\frac{\beta_{z_j}}{\alpha_{z_j}} = \frac{v_{s_b} \cos\left(\alpha_{z_j} \frac{L_z}{2}\right) - D_{\text{eff}} \alpha_{z_j} \sin\left(\alpha_{z_j} \frac{L_z}{2}\right)}{v_{s_b} \sin\left(\alpha_{z_j} \frac{L_z}{2}\right) + D_{\text{eff}} \alpha_{z_j} \cos\left(\alpha_{z_j} \frac{L_z}{2}\right)} \quad (51)$$

This ratio determines the expression of the eigenmodes

$$v_j(z) = \cos(\alpha_{z_j} z) + \frac{\beta_{z_j}}{\alpha_{z_j}} \sin(\alpha_{z_j} z) \quad (52)$$

if the eigenvalues,  $\alpha_{z_j}^2$ , are known. We note that for symmetric boundary conditions,  $v_{s_b} = v_{s_t} = v_s$ , Eq. 44 implies  $\beta_{z_j}/\alpha_{z_j} = 0$ , and the eigenmodes reduce to cosine functions (cf. Eq. 42).

In the general case of  $v_{s_b} \neq v_{s_t}$ , we proceed to enforce the boundary condition at the top surface, which leads to

$$D_{\text{eff}} \left[ \alpha_{z_j} \alpha_{z_j} \sin\left(\alpha_{z_j} \frac{L_z}{2}\right) - \beta_{z_j} \alpha_{z_j} \cos\left(\alpha_{z_j} \frac{L_z}{2}\right) \right] = v_{s_t} \left[ \alpha_{z_j} \cos\left(\alpha_{z_j} \frac{L_z}{2}\right) + \beta_{z_j} \sin\left(\alpha_{z_j} \frac{L_z}{2}\right) \right] \quad (53)$$

Upon insertion of Eq. 51, we readily find

$$\frac{D_{\text{eff}} \alpha_{z_j} \sin(\alpha_{z_j} \frac{L_z}{2}) - v_{s_t} \cos(\alpha_{z_j} \frac{L_z}{2})}{D_{\text{eff}} \alpha_{z_j} \cos(\alpha_{z_j} \frac{L_z}{2}) + v_{s_t} \sin(\alpha_{z_j} \frac{L_z}{2})} = - \frac{D_{\text{eff}} \alpha_{z_j} \sin(\alpha_{z_j} \frac{L_z}{2}) - v_{s_b} \cos(\alpha_{z_j} \frac{L_z}{2})}{D_{\text{eff}} \alpha_{z_j} \cos(\alpha_{z_j} \frac{L_z}{2}) + v_{s_b} \sin(\alpha_{z_j} \frac{L_z}{2})} \quad (54)$$

For symmetric boundary conditions, Eq. 54 reduces to Eq. 44, as expected. For  $v_{s_b} \neq v_{s_t}$ , instead, we arrive (after some algebra) at

$$\cot(\alpha_{z_j} L_z) = \frac{D_{\text{eff}}^2 (\alpha_{z_j} L_z)^2 - v_{s_t} v_{s_b} L_z^2}{D_{\text{eff}} (\alpha_{z_j} L_z) (v_{s_t} + v_{s_b}) L_z} \quad (55)$$

which determines the eigenvalues. The equation is readily solvable, graphically or numerically.

To compute the carrier density, we only need to determine the  $A_{z_j}$  coefficients, for which Eq. 41 still holds. Upon insertion of Eq. 52, we find

$$A_{z_j} = \frac{2\alpha_{z_j} \int_{L_z} \left[ \cos(\alpha_{z_j} z) + \frac{\beta_{z_j}}{\alpha_{z_j}} \cos(\alpha_{z_j} z) \right] F_z(z) dz}{\alpha_{z_j} L_z + \sin(\alpha_{z_j} L_z) + \frac{\beta_{z_j}^2}{\alpha_{z_j}^2} [\alpha_{z_j} L_z - \sin(\alpha_{z_j} L_z)]} \quad (56)$$

which correctly reduces to Eq. 43 for symmetric boundary conditions.

- 
- [1] J. P. McKelvey, *Solid State and Semiconductor Physics* (Robert Kreiger Publ. Co., 1966).
  - [2] G. Moille, S. Combri , and A. De Rossi, Phys. Rev. A **94**, 023814 (2016).
  - [3] G. Moille, S. Combri , K. Fuchs, M. Yacob, J. P. Reithmaier, and A. de Rossi, Opt. Lett. **42**, 795 (2017).
  - [4] K. F. Riley and M. P. Hobson, *Essential Mathematical Methods for the Physical Sciences* (Cambridge University Press, 2011).
  - [5] P. E. Barclay, K. Srinivasan, and O. Painter, Opt. Express **13**, 801 (2005).
  - [6] Y. Yu, E. Palushani, M. Heuck, N. Kuznetsova, P. T. Kristensen, S. Ek, D. Vukovic, C. Peucheret, L. K. Oxenl we, S. Combri , A. de Rossi, K. Yvind, and J. M rk, Opt. Express **21**, 31047 (2013).
  - [7] G. Moille, S. Combri , L. Morgenroth, G. Lehoucq, F. Neuilly, B. Hu, D. Decoster, and A. de Rossi, Laser & Photonics Reviews **10**, 409 (2016).
  - [8] T. J. Johnson, M. Borselli, and O. Painter, Opt. Express **14**, 817 (2006).
  - [9] T. Otaredian, Solid-State Electronics **36**, 153 (1993).
  - [10] M. Maiberg and R. Scheer, Journal of Applied Physics **116**, 123711 (2014).
